# Supplementary material for: Semantic Noise Reduction via Teacher-Guided Dual-Path Audio-Visual Representation Learning
Source: arXiv:2604.08147 source file (2026-04-09)
Supplement: Supplementary file 1 [file X_suppl.tex]

\clearpage
\setcounter{page}{1}
\maketitlesupplementary

\section{Additional Experimental Details}
\subsection{Baseline Architectural Summary}

For completeness, we provide implementation-level details of the
CAV-MAE Sync backbone that are not fully described in the main paper.
These clarify how the baseline organizes tokens, routes information,
and separates objectives during training.
\paragraph{Token Organization.}
For each modality, CAV-MAE Sync prepends:
(i) a \emph{dedicated global token} used exclusively for the contrastive pathway, and
(ii) a set of \emph{register tokens} that act as intermediate buffers within the transformer.
These tokens do not participate in patch reconstruction.
Instead, they stabilize the attention flow and prevent patch tokens from absorbing
semantic responsibilities needed for contrastive learning.
\paragraph{Joint-Layer Execution Structure.}
Unlike the original CAV-MAE, Sync performs \emph{three forward passes}
through the joint transformer layer $J$, each with its own LayerNorm:
\begin{itemize}
    \item visual-only pass: $J_v(Z^v)$,
    \item audio-only pass: $J_a(Z^a)$,
    \item fused pass for reconstruction: $J_{\text{fuse}}([\mathrm{vis}(Z^v);\mathrm{vis}(Z^a)])$.
\end{itemize}
The first two passes generate modality-specific global representations
\emph{without} involving masked tokens.
The fused pass is used only by the reconstruction decoder.

\paragraph{Global Token Pathway.}
The global tokens are not averaged from patches (as in MAE and CAV-MAE).
Instead, after the single-modality encoders,
the global token is fed directly into its corresponding joint-layer pass:
\[
g^{v} = \mathrm{LN}_v(J_v(Z^v)_0), \qquad
g^{a} = \mathrm{LN}_a(J_a(Z^a)_0),
\]
where the subscript $0$ denotes the global-token position.
This ensures that contrastive learning operates on explicitly learned
semantic tokens rather than statistics of visible patches.

\paragraph{Reconstruction Pathway.}
Only \emph{visible patch tokens} are forwarded to $J_{\text{fuse}}$.
Global tokens and register tokens are \emph{removed} from the reconstruction stream.
This prevents gradients from the generative objective from flowing
through global tokens and interfering with cross-modal alignment.
The joint decoder $D$ receives a concatenation of reconstructed visual and audio
features and predicts masked patches for \emph{both} modalities.

\paragraph{Masking Semantics.}
CAV-MAE Sync applies independent random masks to visual and audio patches.
Because global tokens do not depend on masked inputs,
their gradients are unaffected by the stochastic patch visibility,
reducing semantic noise compared to CAV-MAE where global descriptors
are aggregated from partially visible patches.

\paragraph{Temporal Handling.}
A key difference from the standard CAV-MAE baseline is that Sync
treats audio as a sequence aligned to the $T$ sampled video frames.
The baseline therefore generates:
\begin{itemize}
    \item $T$ audio segments (one per frame),
    \item $T$ audio global tokens,
    \item $T$ visual global tokens,
\end{itemize}
enabling multi-token temporal contrast without modifying the backbone architecture.

\subsection{Data Preprocessing}

We follow the official CAV-MAE Sync preprocessing pipeline without modification. Each video is uniformly sampled into $T{=}16$ frames, which are resized and center-cropped to $224{\times}224$ before being patchified into $16{\times}16$ visual patches. The corresponding audio waveform is converted into 128-bin log-Mel filterbanks using a 25\,ms Hanning window and 10\,ms hop. For every sampled frame, a temporally aligned 4-second spectrogram segment (size $128{\times}416$) is extracted by mapping the frame index to its spectrogram coordinate, ensuring strict frame-level temporal correspondence. These audio segments are then patchified with the same $16{\times}16$ grid, producing $208$ audio tokens per segment. Standard normalization is applied to both modalities, and the resulting sequences serve as the input token streams for subsequent masking and encoding in the baseline model.

In practice, to reduce I/O overhead during large-scale pretraining, we additionally package all audio-visual samples into \texttt{webdataset} shards. Each shard stores paired RGB frames, their aligned audio segments, and the corresponding metadata, enabling sequential and locality-friendly reads during distributed training. This packaging significantly alleviates random-access bottlenecks inherent to filesystem-based loading, allowing the dataloader to stream pre-compressed samples efficiently across multiple GPUs and improving overall training throughput.

\noindent
\begin{minipage}{1\linewidth}
\small
\raggedright
\setlength{\tabcolsep}{3.5pt}
\begin{tabular}{lccc}
\toprule
\textbf{Setting} & \textbf{Pretrain} & \textbf{AS20K LP} & \textbf{VGG LP} \\
\midrule
Dataset & AS-2M & AS-20K & VGGSound \\
Optimizer & Adam & Adam & Adam \\
Learning Rate & $2\!\times\!10^{-4}$ & $5\!\times\!10^{-2}$ & $1\!\times\!10^{-3}$ \\
LR Scheduler & Cosine & Cosine & Cosine \\
Epochs & \textbf{35} & 15 & 10 \\
Warmup Epochs & \textbf{3.5} & 1.5 & 1 \\
Batch Size & $8\times 64$ & 48 & 48 \\
GPUs & \textbf{8$\times$H100} & 2$\times$H100 & 2$\times$H100 \\
Audio Input Size & 128$\times$416 & $16\times$128$\times$416 & $16\times$128$\times$416 \\
Class-Balanced & No & No & Yes \\
Mixup & No & Yes & Yes \\
Random Shift & Yes & Yes & Yes \\
Loss Function & --- & BCE & CE \\
Weight Averaging & No & Yes & Yes \\
Norm Mean & $-5.081$ & $-5.081$ & $-5.081$ \\
Norm STD & 4.485 & 4.485 & 4.485 \\
\bottomrule
\end{tabular}
\captionof{table}{Hyperparameters for pretraining and linear probing.}
\label{tab:pretrain-lp}
\end{minipage}

\subsection{Pretraining Configuration}

Our pretraining setup follows the official CAV-MAE Sync configuration, including optimizer settings, masking ratio, data augmentations, batch size, and loss weights. All experiments are conducted on 8$\times$\,NVIDIA H100 GPUs. Due to missing entries in our local AudioSet-2M copy, we extend the pretraining schedule from 25 to 35 epochs, and proportionally adjust warmup and cosine learning-rate scheduling. Refer to ~\ref{tab:pretrain-lp} for detailed configurations.

Although our dual-path framework introduces an additional teacher forward pass, the extra computation is modest because the teacher processes only short sequences. In practice, the per-epoch time increases from 730\,s to 1045\,s, resulting in a total pretraining time of approximately 7.1\,h. Table~\ref{tab:time-comparison} summarizes this overhead.

\begin{table}[h]
\centering
\setlength{\tabcolsep}{10pt}
\begin{tabular}{lcc}
\toprule
\textbf{Model} & \textbf{Per-epoch (s)} & \textbf{Total } \\
\midrule
baseline & 730  & 7.1 h \\
Ours          & 1045 & 10.2 h \\
\bottomrule
\end{tabular}
\caption{Pretraining runtime comparison. The dual-path teacher branch increases cost moderately while remaining efficient.}
\label{tab:time-comparison}
\end{table}

\subsection{Downstream Evaluation}

For all downstream tasks, we keep the implementation consistent with the original CAV-MAE Sync settings to ensure comparability. This includes the same optimizer (Adam with $(\beta_1, \beta_2)=(0.95, 0.999)$), cosine learning-rate schedule with warmup, masking strategy, and lightweight data augmentations applied during linear probing. Unless otherwise specified, all encoder weights are frozen and only the task-specific heads are trained.

\paragraph{Zero-shot Retrieval.}
Since retrieval is not fully detailed in the main paper, we summarize the procedure here. For each video, the model produces a temporal sequence of visual and audio global tokens, $\{g_t^v\}_{t=1}^T$ and $\{g_t^a\}_{t=1}^T$. For any query–candidate pair, a $T{\times}T$ cosine-similarity matrix is computed between these sequences. The final similarity score is obtained by averaging the diagonal elements, which corresponds to comparing frame-aligned audio–visual tokens. This score is used to rank candidates, and Recall@$\{1,5,10\}$ is reported for both V$\rightarrow$A and A$\rightarrow$V retrieval on the standard subsampled splits.

\paragraph{Classification.}
For AudioSet-20K and VGGSound classification, we train only the two-layer classification head while keeping the pretrained encoders fixed. We use binary cross-entropy for AudioSet and standard cross-entropy for VGGSound. The same sampling strategy, data normalization, and mixup settings as in the original configuration are used. The learning rate follows a cosine schedule with task-dependent peak values.

\section{Visualization and Qualitative Analysis}
\subsection{Training Dynamics Analysis}

Figure~\ref{fig:dynamic} compares the training behavior of the original 
CAV-MAE Sync baseline with our dual-path formulation. We report the per-step reconstruction 
loss and contrastive loss throughout pretraining. A clear pattern emerges: in both models, 
the reconstruction objective converges extremely quickly, stabilizing within the first few 
hundred iterations. In contrast, the contrastive objective decreases at a significantly slower 
rate and continues to improve for thousands of steps. This divergence in optimization speed 
suggests that the generative and discriminative objectives are only weakly coupled during 
training and naturally evolve on different timescales.

This observation supports the rationale behind our decoupling strategy: since reconstruction 
and alignment exhibit largely independent behaviors, optimizing them in separate pathways is 
a principled choice. Moreover, the dual-path design accelerates the optimization of the 
contrastive branch, as shown by the consistently faster decay of the contrastive loss in our 
model. By preventing gradient interference and ensuring both pathways receive clean, 
unconflicted supervision signals, the dual-path formulation enables more stable optimization 
and faster convergence, particularly for the alignment objective that directly drives 
cross-modal semantic learning.

We additionally observe a consistent gap between the reconstruction losses of the two
modalities: both the baseline and our dual-path model stabilize around a vision
reconstruction loss of approximately $0.35$, whereas the audio reconstruction loss
remains notably higher at roughly $0.60$. This discrepancy indicates that the model
finds it substantially easier to encode and reconstruct visual tokens than audio
tokens, reflecting the stronger spatial structure and inductive biases inherent to
vision Transformers. As discussed in the main paper, this imbalance suggests that
cross-modal interaction is often visually anchored, with the model more readily
leveraging visual representations during alignment and downstream tasks. The
consistent reconstruction gap highlights an intrinsic asymmetry between modalities
and further motivates architectural designs that prevent the visually dominant
representations from overwhelming the audio pathway during joint learning.

\subsection{Cross-Modal Retrieval Case Study}
To better understand the qualitative advantages of our approach, 
Figure~\ref{fig:retr} presents a cross-modal retrieval case study comparing 
the top retrieved videos from the baseline CAV-MAE Sync and our method 
under various audio queries. Each row corresponds to a distinct sound event, 
including \emph{roller coaster running}, \emph{people shuffling}, 
\emph{basketball bounce}, and \emph{dog barking}. 

Across all examples, the baseline often returns videos that share only 
coarse or incidental correlations with the audio query (e.g., unrelated 
scenes with background noise or visually mismatched contexts). 
This behavior reflects the limitations of global audio representations and 
coupled reconstruction-contrastive optimization, which tend to dilute 
fine-grained semantic cues necessary for discriminative retrieval.
In contrast, our method consistently retrieves videos whose visual content 
closely matches the semantics and temporal characteristics of the input audio.

\subsection{Global Token Embedding Visualization}
To qualitatively assess the semantic structure of the learned representations,
we project the audio and video global tokens into a shared 2D space using t-SNE.
We randomly sample 10 classes from the VGGSound test split and 
encode both modalities with the pretrained models.
Audio and video embeddings are visualized using distinct marker shapes 
(circles for audio, triangles for video), while colors indicate different semantic categories.

As shown in Fig.~\ref{fig:tsne}, the baseline model exhibits noticeable modality discrepancy:
audio and video embeddings belonging to the same class are distributed across distant regions,
and the resulting clusters often display weak semantic coherence.
This misalignment reflects the inherent limitations of joint reconstruction-alignment
optimization, where random masking and inconsistent gradients introduce semantic noise.

In contrast, our method produces markedly tighter structures.
Audio and video embeddings of the same class form compact, well-overlapped co-clusters,
while clusters of different classes become more clearly separated.
These improvements confirm that our teacher-guided dual-path framework
successfully enhances global semantic alignment, enabling the model to learn 
a more modality-consistent and discriminative embedding space.
\begin{figure*}[t]
    \centering
    \includegraphics[width=\textwidth]{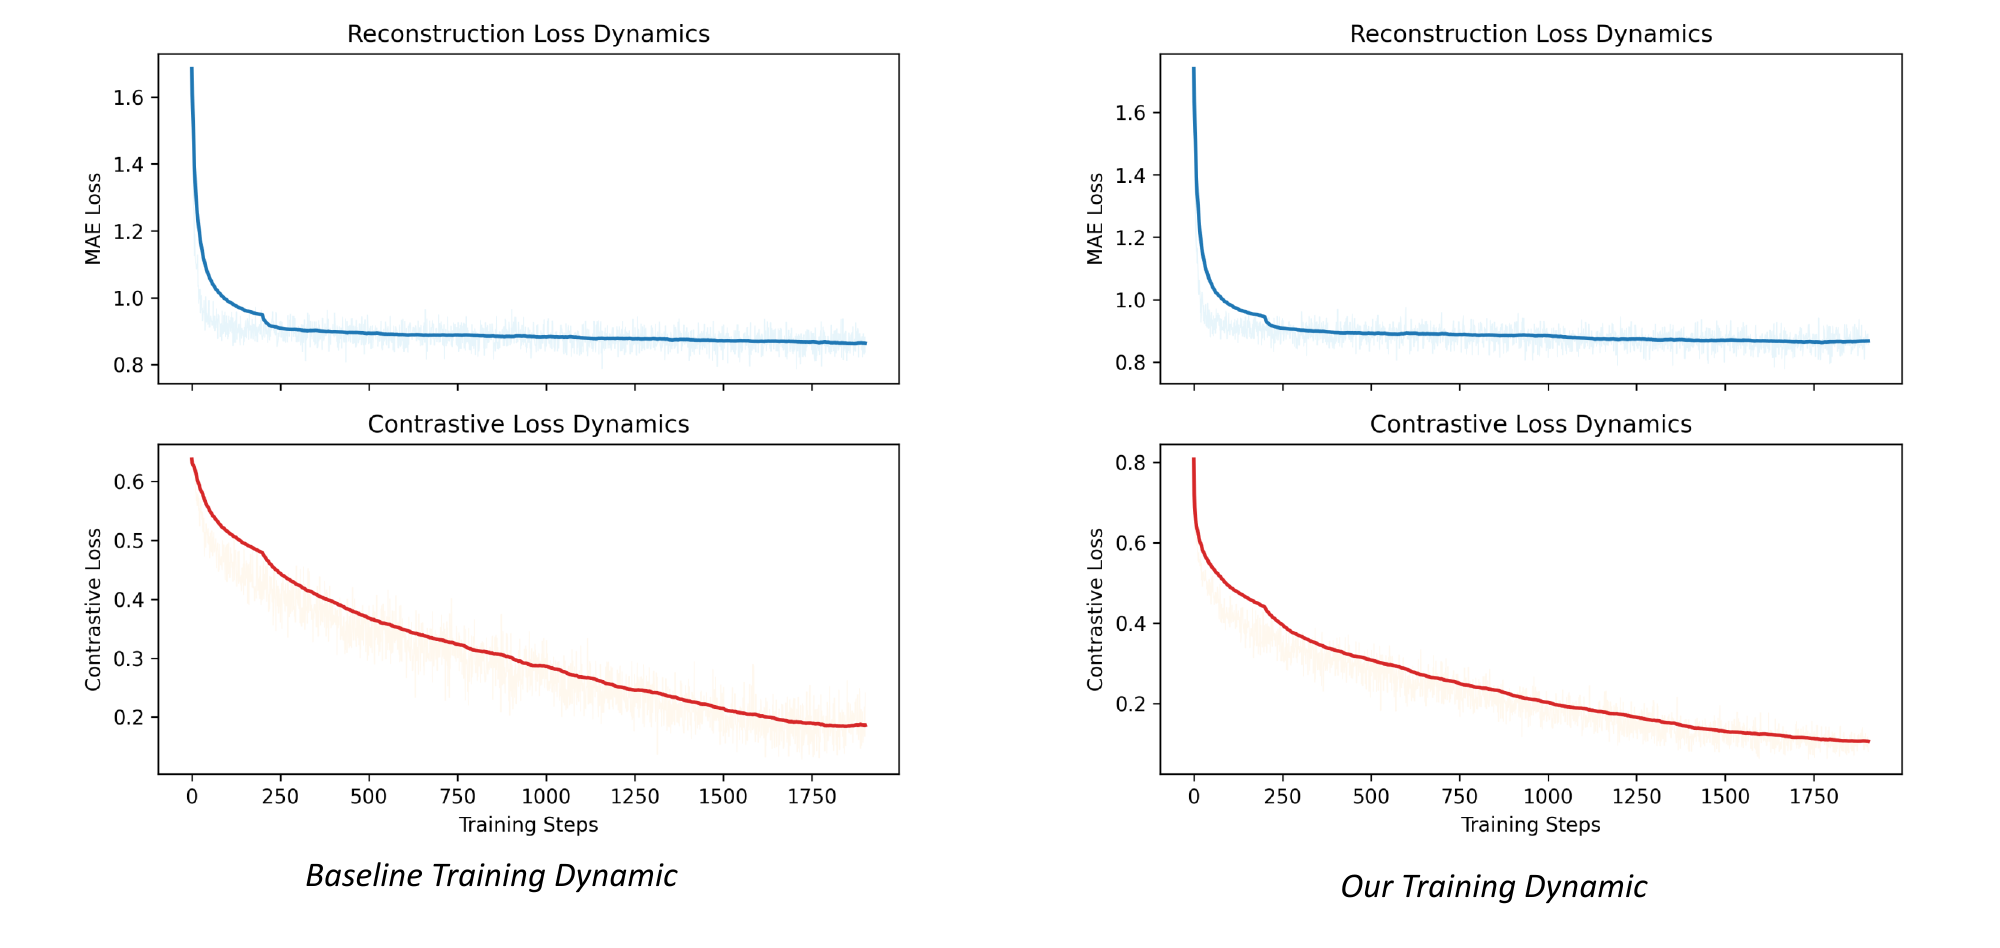}
    \caption{
Training loss dynamics of the baseline CAV-MAE Sync (left) and our dual-path formulation (right). 
For both models, the reconstruction loss quickly converges within the first few hundred steps, 
while the contrastive loss decreases much more slowly, indicating that the two objectives behave 
largely independently during optimization. Our dual-path strategy further accelerates the 
convergence of the contrastive branch, supporting the motivation of separating reconstruction 
and alignment pathways for more stable and efficient training.
}
    \label{fig:dynamic}
\end{figure*}

\begin{figure*}[t]
    \centering
    \includegraphics[width=\textwidth]{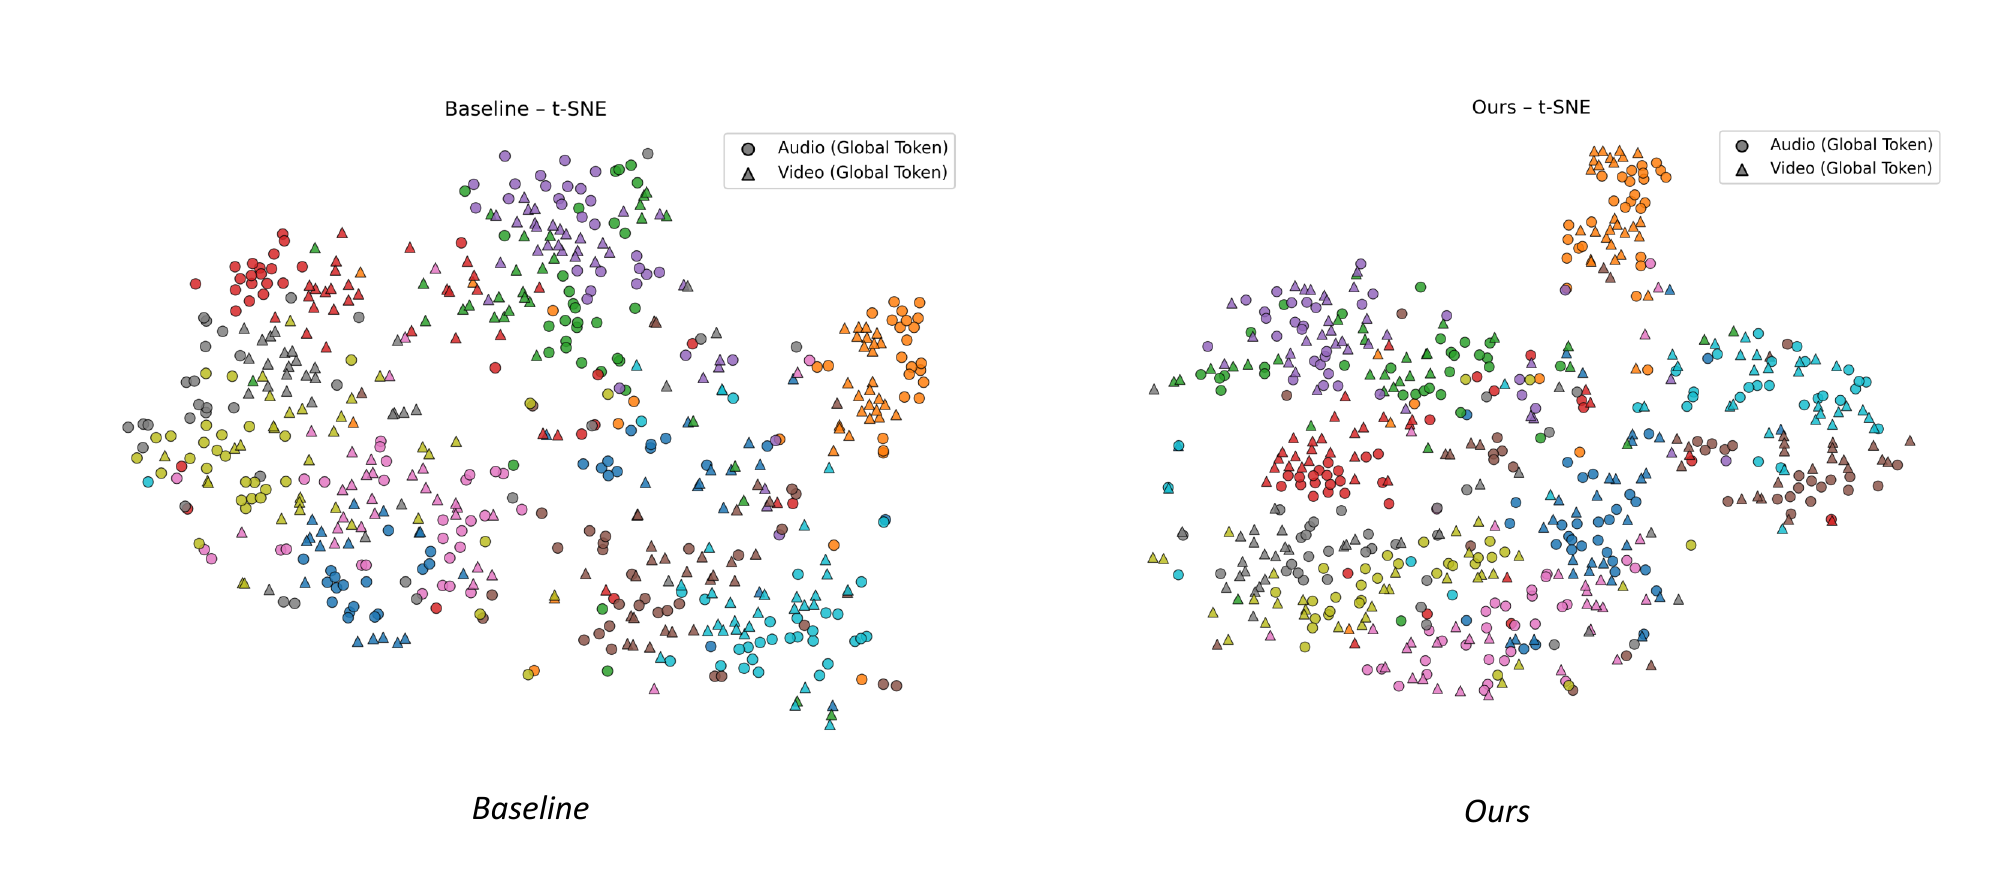}
    \caption{
    t-SNE visualization of global token embeddings from the baseline (left) and our method (right).
    Each point denotes a global embedding, with \textbf{circles for audio} and \textbf{triangles for video}, and colors indicating different semantic classes.
    The baseline exhibits modality discrepancy compared to ours. Audio and video clusters of the some class are loosely aligned and often drift apart.
    In contrast, our method produces \textbf{tight audio-video co-clusters} with clearer inter-class separation, demonstrating substantially improved cross-modal consistency learned during pretraining.
}
    \label{fig:tsne}
\end{figure*}

\begin{figure*}[t]
    \centering
    \includegraphics[width=\textwidth]{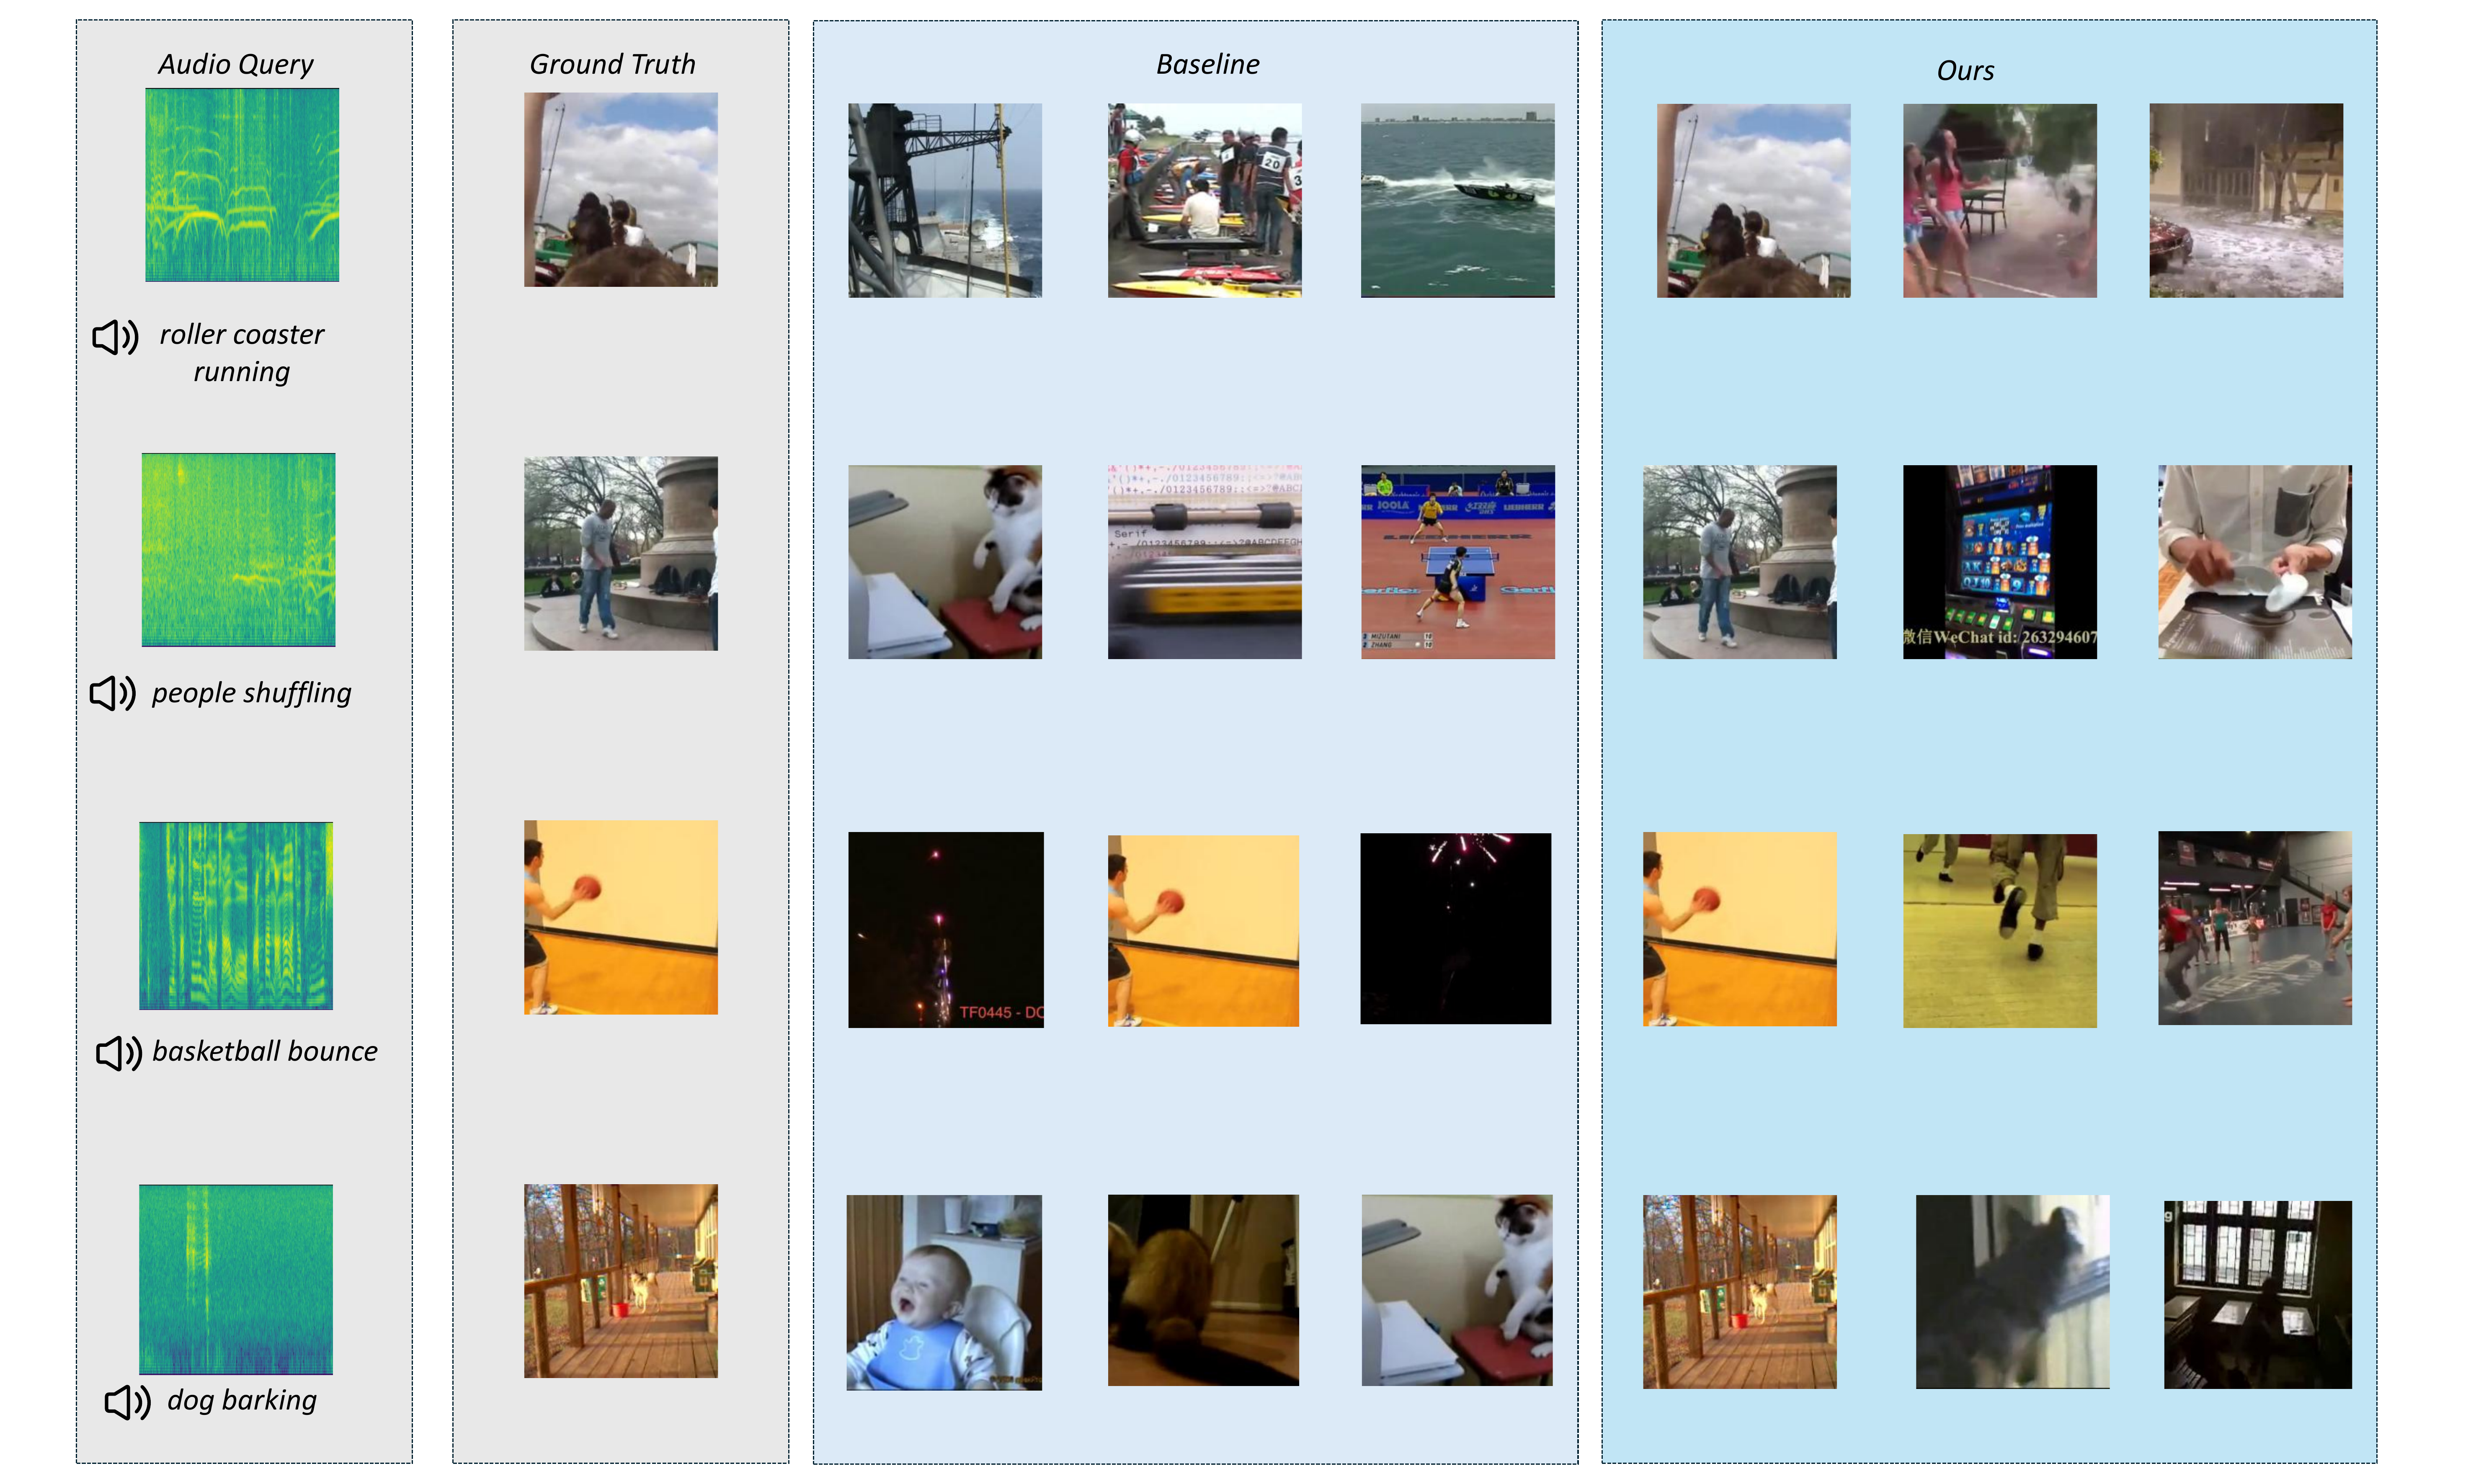}
    \caption{
\textbf{Qualitative cross-modal retrieval results.}
Given an audio query (left), we compare the top retrieved videos from the \textbf{baseline CAV-MAE Sync} (middle) and \textbf{our method} (right).
Each row corresponds to a different audio event (\emph{roller coaster running}, \emph{people shuffling}, \emph{basketball bounce}, \emph{dog barking}).
While the baseline frequently retrieves semantically irrelevant or visually mismatched scenes, our model consistently returns videos that better match both the \emph{sound semantics} and the \emph{visual content}, demonstrating substantially improved audio-visual alignment learned during pretraining.
}
    \label{fig:retr}
\end{figure*}
